# Supplementary material for: Mechanical response of dense pedestrian crowds to the crossing of intruders
Source: arXiv:1810.03343 source file (2018-10-08)
Supplement: Supplementary file 1 [file SuppMat.pdf]

# Supplementary Information for: Mechanical response of dense pedestrian crowds to the crossing of intruders

Alexandre NICOLAS<sup>1,\*</sup>, Marcelo KUPERMAN<sup>2</sup>, Santiago IBÁÑEZ<sup>2,3</sup>, Sebastián BOUZAT<sup>2</sup>, and Cécile APPERT-ROLLAND<sup>4</sup>

<sup>1</sup>LPTMS, CNRS, Université Paris-Sud, Université Paris-Saclay, 91405 Orsay, France.

<sup>2</sup>Consejo Nacional de Investigaciones Científicas y Técnicas, Centro Atómico Bariloche (CNEA) and Instituto Balseiro, R8400AGP Bariloche, Argentina.

<sup>3</sup>Universidad Nacional de Río Negro, Sede Andina, 8400 Bariloche, Argentina.

<sup>4</sup>LPT, CNRS UMR 8627, Université Paris-Sud, Université Paris-Saclay, 91405 Orsay, France.

\*alexandre.nicolas@polytechnique.edu

## ABSTRACT

We provide three additional figures as Supplemental Material.

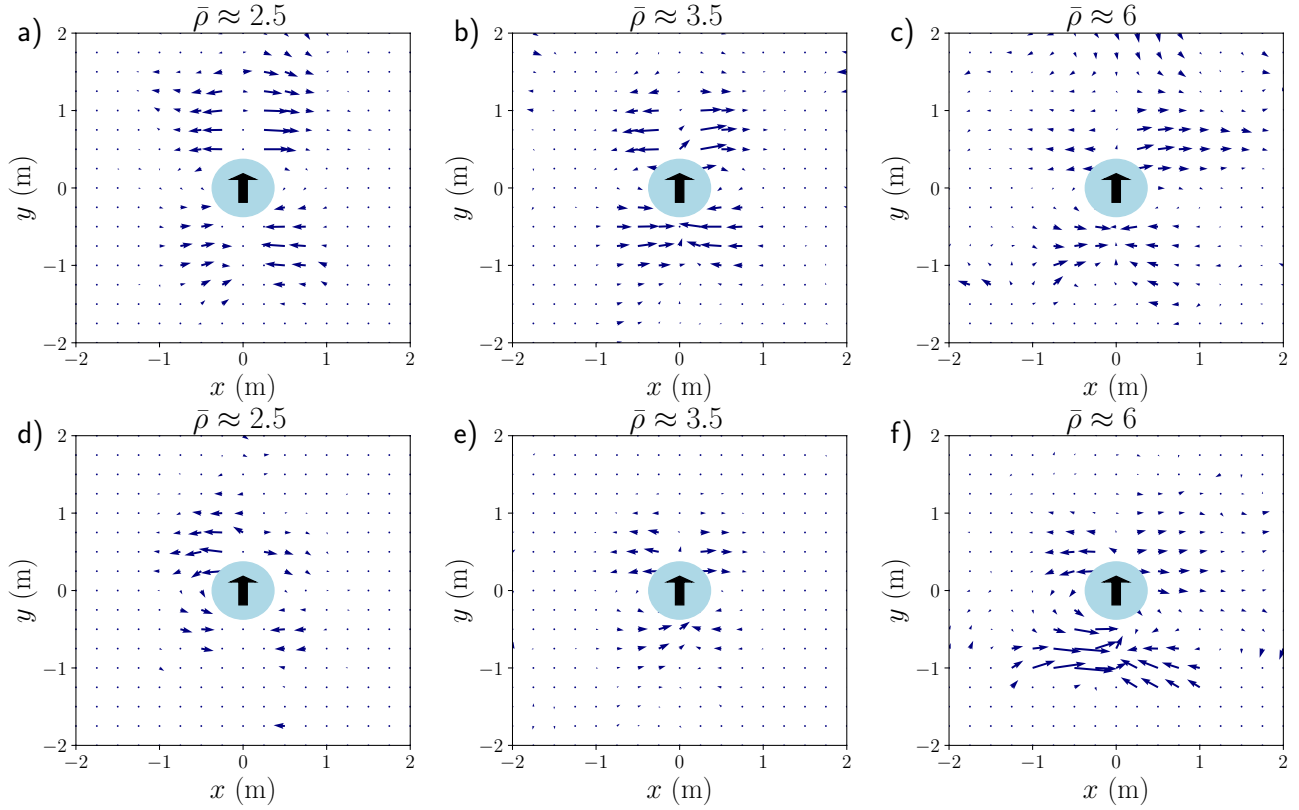

**Figure S1.** Mean velocity fields (based on the displacements over a time window  $\delta t = 0.5$  s) around the cylinder in crowds of participants facing the intruder (top row) and randomly oriented ones (bottom row) at (a-d) moderate density ( $\bar{\rho} \approx 2.5$  ped/m<sup>2</sup>), (b-e) fairly high density ( $\bar{\rho} \approx 3.5$  ped/m<sup>2</sup>), and (c-f) very high density ( $\bar{\rho} \approx 6$  ped/m<sup>2</sup>). The velocity arrows on the left, middle, and right panels are magnified by a factor 1, 2, and 4, respectively.

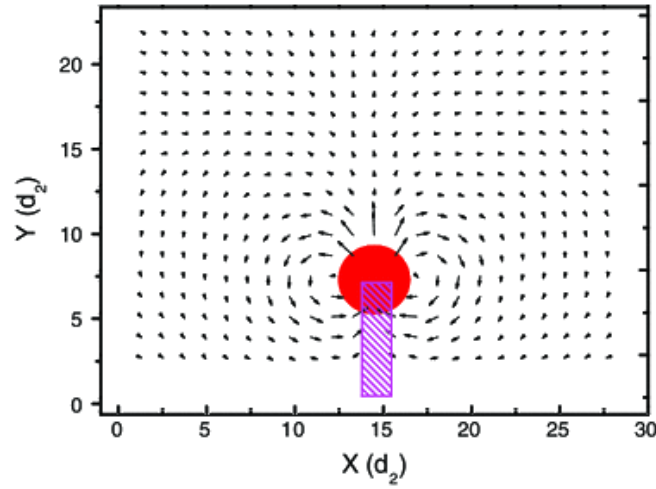

**Figure S2.** Mean velocity field around a circular intruder in a two-dimensional granular medium. Adapted from Ref. <sup>1</sup>, with permission.

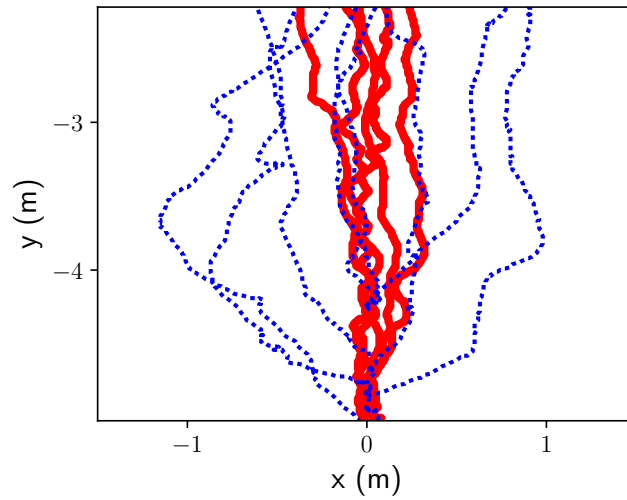

**Figure S3.** Traces of a few typical trajectories of the cylindrical intruder (thick red lines) and of crossing pedestrians (dotted blue lines) through a fairly dense crowd ( $\rho \approx 3.5 \text{ ped/m}^2$ ) facing the intruder. The trajectories have been shifted horizontally to start from  $x = 0$ .

## References

1. Kolb, E., Cixous, P. & Charmet, J. Flow fields around an intruder immersed in a 2d dense granular layer. *Granul. Matter* **16**, 223–233 (2014).
